# Supplementary material for: IQA-Adapter: Exploring Knowledge Transfer from Image Quality Assessment to Diffusion-based Generative Models
Source: arXiv:2412.01794 source file (2025-03-16)
Supplement: Supplementary file 1 [file neg_guidance_supp_old.tex]

\section{Negative Guidance}
\label{sec:neg_guidance}

Since the concept of visual quality has clearly defined notions of "good" and "bad," it becomes feasible to apply \textbf{negative guidance}, akin to its application in text-based generation. Negative guidance for text involves using an additional text prompt that is semantically opposite to the desired outcome. This serves as a conditioning factor in the unconditional part of the generation process:
\begin{equation*}
    \hat{\epsilon}_\theta (z_{t}|c_t, q) 
        = \epsilon_{\theta}(z_t| \varnothing)
        + g \cdot \big(
            \epsilon_{\theta}(z_t| c_t, q)
            - \epsilon_{\theta}(z_t| \varnothing)
        \big)
\end{equation*}
where $\epsilon_{\theta}$ is a latent diffusion model, $g$ is guidance scale, $c_t$ is a textual condition, $q$ is desired quality of image and $\varnothing$ is an empty condition.

This approach pushes the latent representation of the generated image away from producing undesired features described in the negative prompt. 

The standard method for using an IP-Adapter assumes a null-condition in the unconditional part of the noise prediction, as there is no explicit counter-concept for an image prompt. The task of quality conditioning, however, enables defining negative guidance as:
\begin{multline*}
    \hat{\epsilon}_\theta (z_{t}|c_t, q) 
    = \epsilon_{\theta}(z_t| c_t^{\text{neg}}, q^{\text{neg}})
    +  \\
    + g \cdot \big(
        \epsilon_{\theta}(z_t| c_t, q)
        - \epsilon_{\theta}(z_t| c_t^{\text{neg}}, q^{\text{neg}})
    \big)
\end{multline*}
where $q^{\text{neg}}$ specifies a quality level opposite to the desired one and $c_t^{\text{neg}}$ is negative prompt. Since the input scores are normalized with a mean of 0, we can set \(q^{\text{neg}} = -q\). 

Using this approach enhances the adapter's effect, even with moderate adapter strengths. The resulting images become more vivid, sharp, and, in a sense, stylized to align with the ideals of the target metric. Examples of applying negative guidance with various types of negative conditions are presented in Figure~\ref{fig:neg_guidance_good_example}.

Strong negative guidance significantly improves metric scores, with generalization across different metrics. Figure~\ref{fig:neg_guidance_heatmap} shows average improvements increasing from 5-6\% to 8-10\% relative to the base model.
However, strong negative guidance with high adapter scales can result in overly clean, saturated, sharp images, losing fine details (Figure~\ref{fig:neg_guidance_example_supp}). This effect intensifies with higher scales.

These findings emphasize the need for subjective validation, as IQA/IAA models may have biases or vulnerabilities, especially in adversarial scenarios. The generalization of quality improvements suggests shared biases among models, similar to vulnerabilities identified in the VMAF IQA metric~\cite{vmaf, hackvmaf1, Zvezdakova2019HackingVW}. 


\begin{figure*}[ht!]
\centering
%\resizebox{.8\textwidth}{}{%
   \includegraphics[width=.98\textwidth]{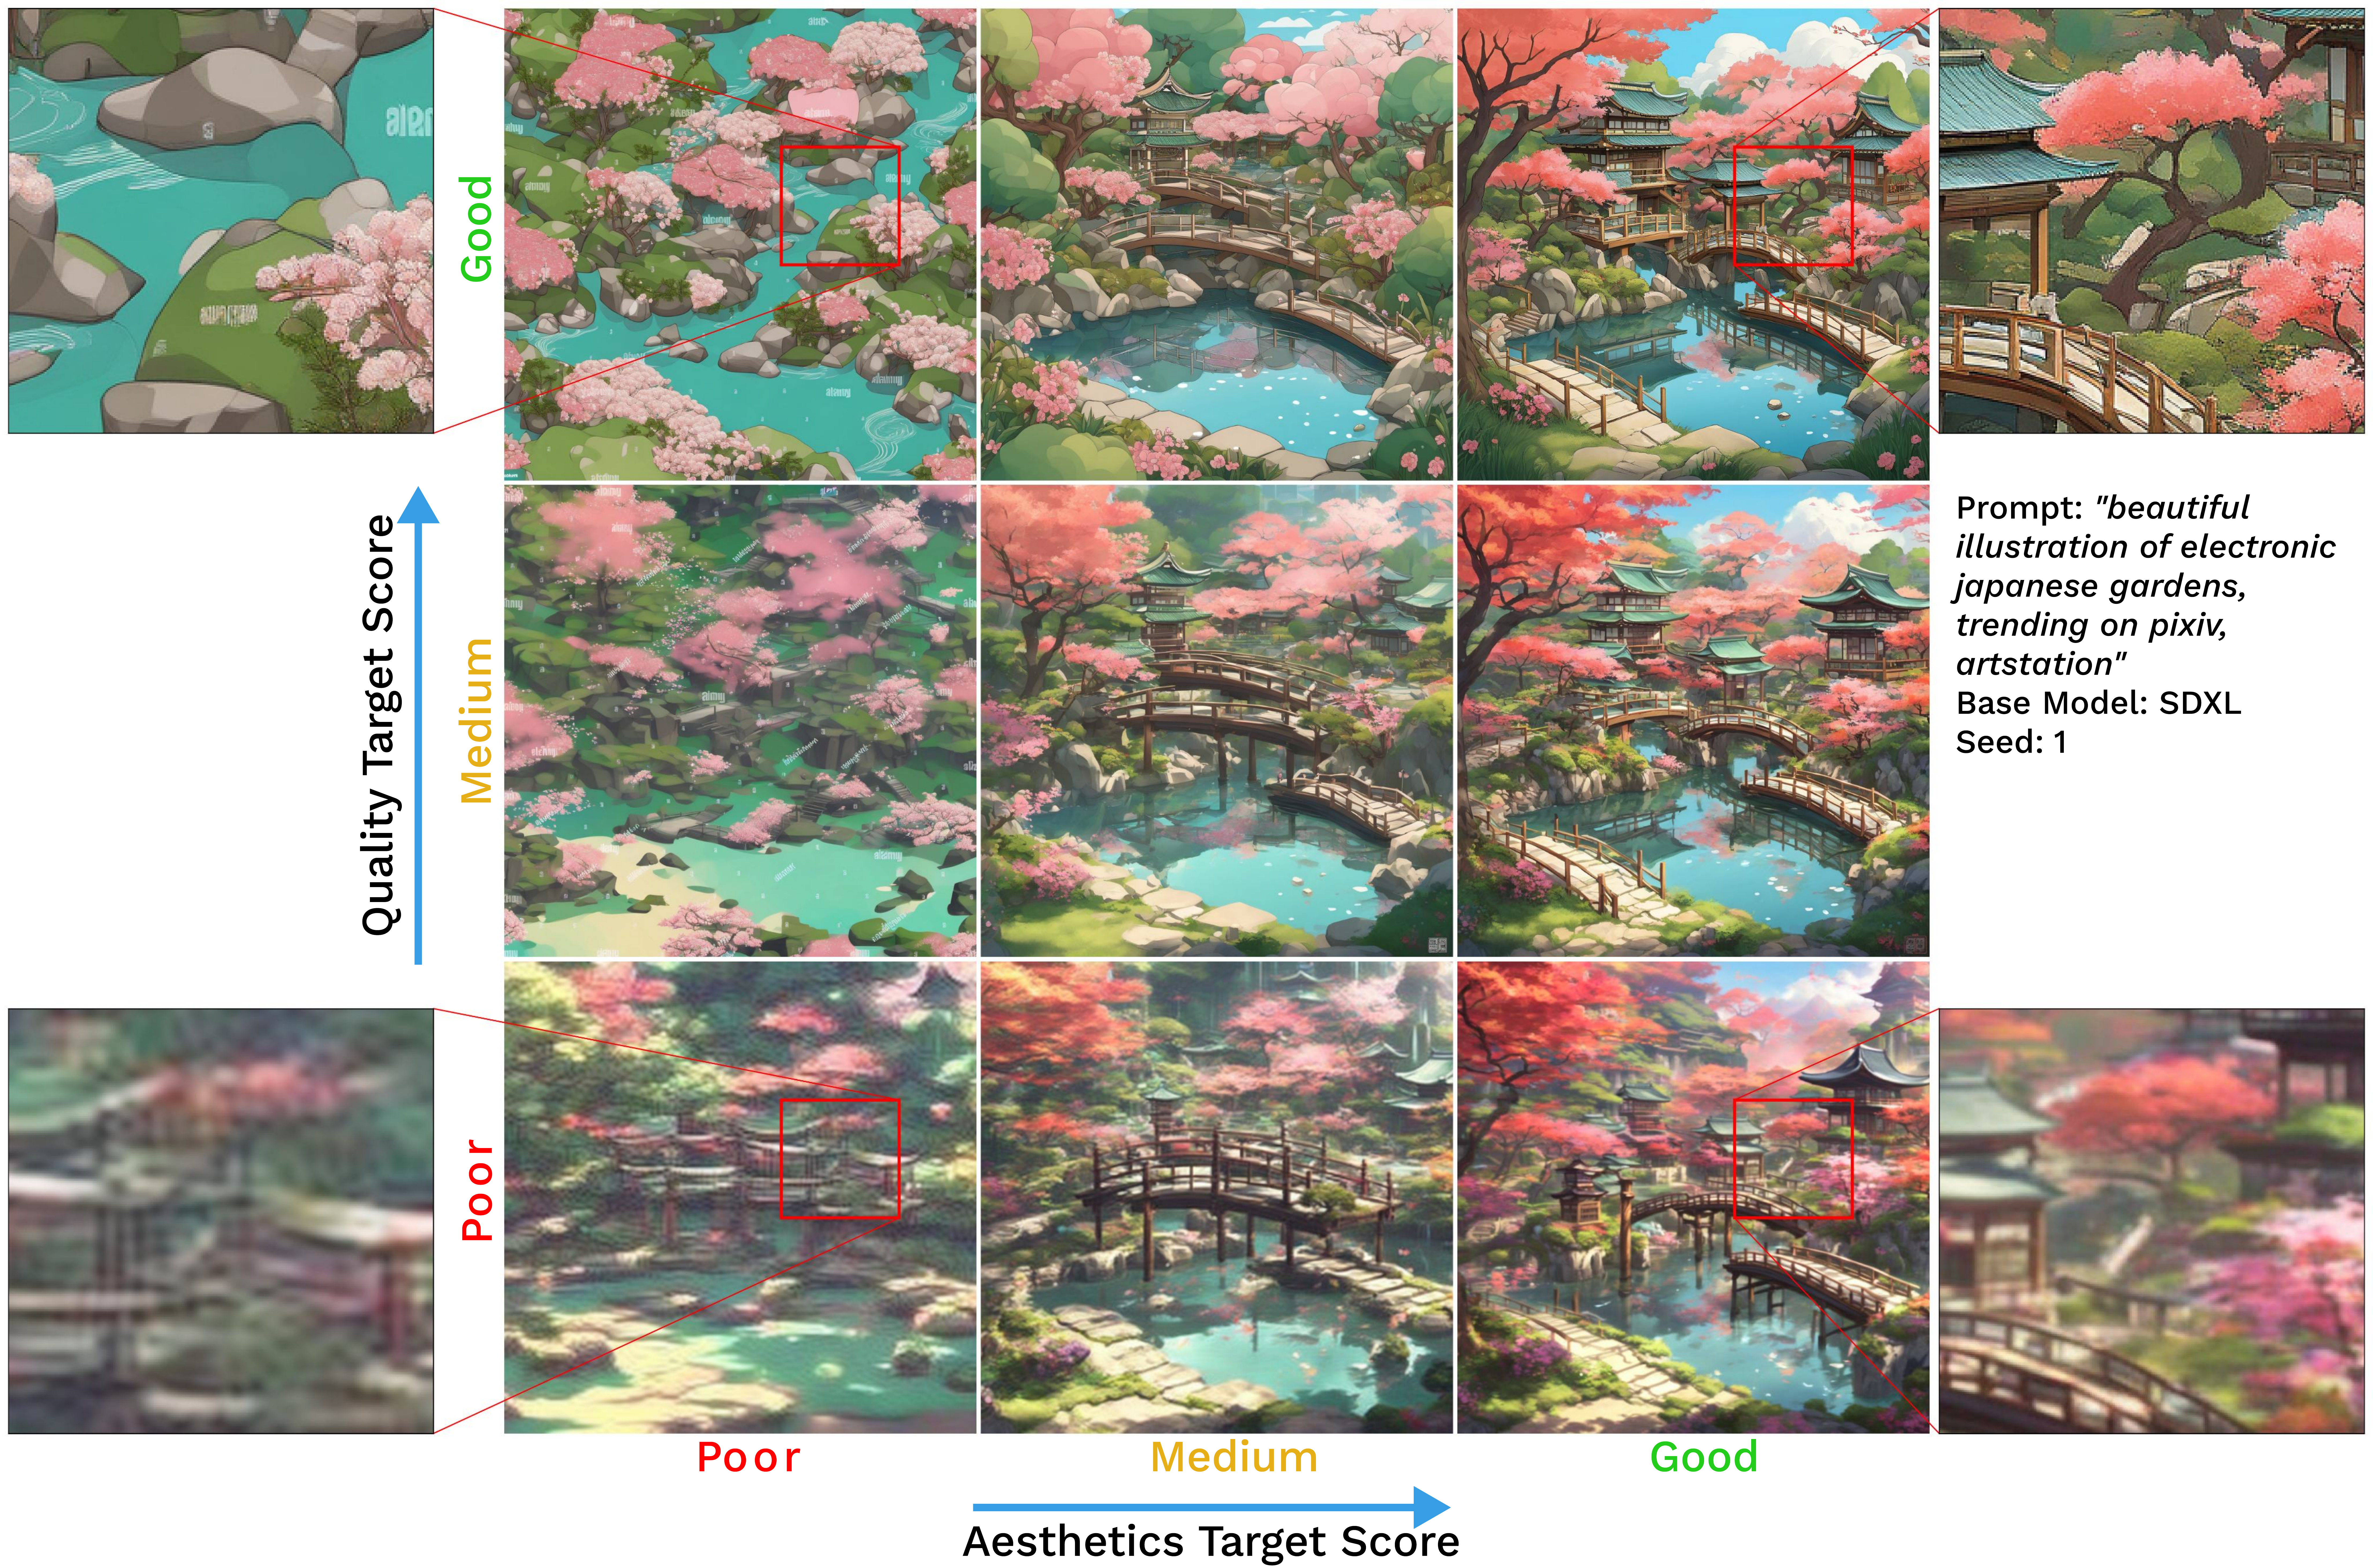}
  \caption{Quality-aware image generation using IQA-Adapter combined with negative guidance. Compared to Figure \ref{fig:demo_2d}, negative guidance exhibits stronger conditioning effect.}
  \label{fig:neg_guidance_good_example}%
%}
\end{figure*}
